# Supplementary material for: Analyzing Semantic Change through Lexical Replacements
Source: arXiv:2404.18570 source file (2024-04-29)
Supplement: Supplementary file 1 [file appendix.tex]

\section{Self-embedding distance (SED)}
 \begin{minipage}{\textwidth}
 \centering
    \includegraphics[width=\textwidth]{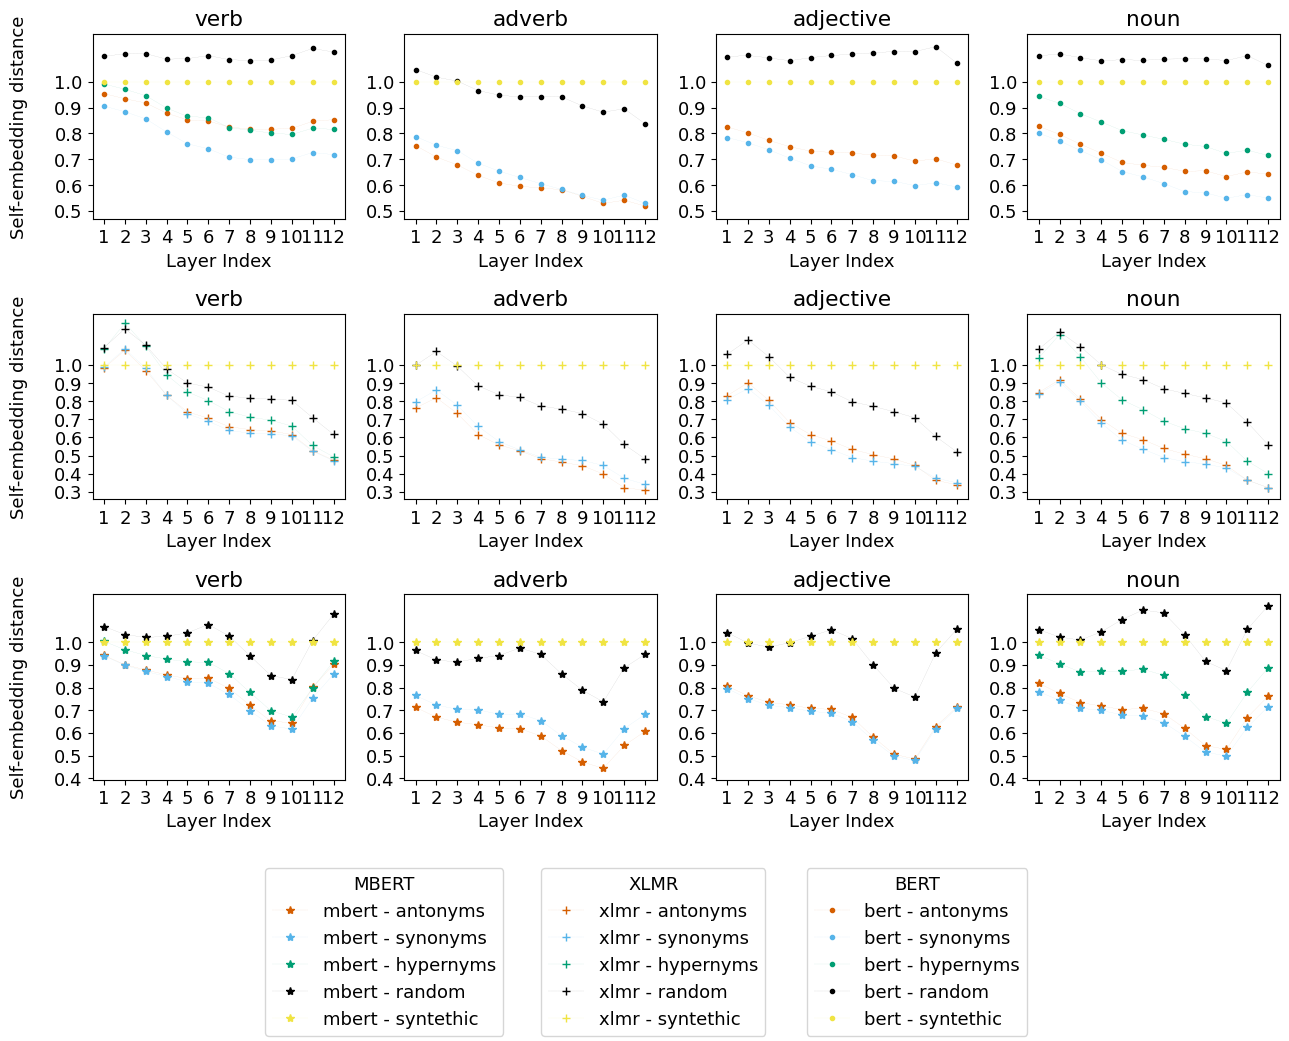}
    \captionof{figure}{Average SED over layers}
    \label{fig:full-self-embedding-distance}
 \end{minipage}

\clearpage

 \begin{table*}
\centering
\resizebox{0.9\textwidth}{!}{%
\begin{tabular}{cccccccccccccccccccc}
 &
   &
  \multicolumn{3}{c}{\textbf{WiC-en}} &
  \multicolumn{3}{c}{\textbf{MCL-WiC-en}} &
  \multicolumn{3}{c}{\textbf{XL-WiC-fr}} &
  \multicolumn{3}{c}{\textbf{XL-WiC-it}} &
  \multicolumn{3}{c}{\textbf{WiC-ITA-it}} &
  \multicolumn{3}{c}{\textbf{DWUG-de}} \\ \cline{3-20} 
 &
  \multicolumn{1}{c|}{Instances} &
  \textit{Dev} &
  \textit{Train} &
  \multicolumn{1}{c|}{\textit{Test}} &
  \textit{Dev} &
  \textit{Train} &
  \multicolumn{1}{c|}{\textit{Test}} &
  \textit{Dev} &
  \textit{Train} &
  \multicolumn{1}{c|}{\textit{Test}} &
  \textit{Dev} &
  \textit{Train} &
  \multicolumn{1}{c|}{\textit{Test}} &
  \textit{Dev} &
  \textit{Train} &
  \multicolumn{1}{c|}{\textit{Test}} &
  \textit{Dev} &
  \textit{Train} &
  \multicolumn{1}{c|}{\textit{Test}} \\ \cline{2-20} 
\multicolumn{1}{c|}{\multirow{2}{*}{\textbf{nouns}}} &
  \multicolumn{1}{c|}{\textit{TP}} &
  196 &
  1474 &
  \multicolumn{1}{c|}{422} &
  290 &
  2093 &
  \multicolumn{1}{c|}{263} &
  275 &
  \textbf{-} &
  \multicolumn{1}{c|}{261} &
  65 &
  340 &
  \multicolumn{1}{c|}{180} &
  166 &
  1153 &
  \multicolumn{1}{c|}{174} &
  778 &
  2402 &
  \multicolumn{1}{c|}{783} \\
\multicolumn{1}{c|}{} &
  \multicolumn{1}{c|}{\textit{TN}} &
  199 &
  1320 &
  \multicolumn{1}{c|}{409} &
  292 &
  2031 &
  \multicolumn{1}{c|}{265} &
  273 &
  \textbf{-} &
  \multicolumn{1}{c|}{253} &
  62 &
  312 &
  \multicolumn{1}{c|}{180} &
  156 &
  463 &
  \multicolumn{1}{c|}{175} &
  168 &
  465 &
  \multicolumn{1}{c|}{163} \\ \cline{2-20} 
\multicolumn{1}{c|}{\multirow{2}{*}{\textbf{verbs}}} &
  \multicolumn{1}{c|}{\textit{TP}} &
  123 &
  1240 &
  \multicolumn{1}{c|}{278} &
  126 &
  1095 &
  \multicolumn{1}{c|}{149} &
  120 &
  \textbf{-} &
  \multicolumn{1}{c|}{117} &
  34 &
  228 &
  \multicolumn{1}{c|}{115} &
  36 &
  414 &
  \multicolumn{1}{c|}{31} &
  349 &
  1081 &
  \multicolumn{1}{c|}{326} \\
\multicolumn{1}{c|}{} &
  \multicolumn{1}{c|}{\textit{TN}} &
  120 &
  1394 &
  \multicolumn{1}{c|}{291} &
  120 &
  1175 &
  \multicolumn{1}{c|}{149} &
  142 &
  \textbf{-} &
  \multicolumn{1}{c|}{155} &
  37 &
  259 &
  \multicolumn{1}{c|}{116} &
  50 &
  200 &
  \multicolumn{1}{c|}{49} &
  249 &
  680 &
  \multicolumn{1}{c|}{270} \\ \cline{2-20} 
\multicolumn{1}{c|}{\multirow{2}{*}{\textbf{adjectives}}} &
  \multicolumn{1}{c|}{\textit{TP}} &
  \textbf{-} &
  \textbf{-} &
  \multicolumn{1}{c|}{\textbf{-}} &
  78 &
  724 &
  \multicolumn{1}{c|}{76} &
  84 &
  \textbf{-} &
  \multicolumn{1}{c|}{101} &
  \textbf{-} &
  \textbf{-} &
  \multicolumn{1}{c|}{\textbf{-}} &
  46 &
  347 &
  \multicolumn{1}{c|}{27} &
  \textbf{-} &
  \textbf{-} &
  \multicolumn{1}{c|}{\textbf{-}} \\
\multicolumn{1}{c|}{} &
  \multicolumn{1}{c|}{\textit{TN}} &
  \textbf{-} &
  \textbf{-} &
  \multicolumn{1}{c|}{\textbf{-}} &
  80 &
  706 &
  \multicolumn{1}{c|}{68} &
  72 &
  \textbf{-} &
  \multicolumn{1}{c|}{83} &
  \textbf{-} &
  \textbf{-} &
  \multicolumn{1}{c|}{\textbf{-}} &
  38 &
  119 &
  \multicolumn{1}{c|}{25} &
  \textbf{-} &
  \textbf{-} &
  \multicolumn{1}{c|}{\textbf{-}} \\ \cline{2-20} 
\multicolumn{1}{c|}{\multirow{2}{*}{\textbf{ALL}}} &
  \multicolumn{1}{c|}{\textit{TP}} &
  319 &
  2714 &
  \multicolumn{1}{c|}{700} &
  500 &
  4000 &
  \multicolumn{1}{c|}{500} &
  500 &
  \textbf{-} &
  \multicolumn{1}{c|}{500} &
  99 &
  568 &
  \multicolumn{1}{c|}{295} &
  250 &
  1999 &
  \multicolumn{1}{c|}{250} &
  1127 &
  3483 &
  \multicolumn{1}{c|}{1109} \\
\multicolumn{1}{c|}{} &
  \multicolumn{1}{c|}{\textit{TN}} &
  319 &
  2714 &
  \multicolumn{1}{c|}{700} &
  500 &
  4000 &
  \multicolumn{1}{c|}{500} &
  500 &
  \textbf{-} &
  \multicolumn{1}{c|}{500} &
  99 &
  571 &
  \multicolumn{1}{c|}{296} &
  250 &
  806 &
  \multicolumn{1}{c|}{250} &
  417 &
  1145 &
  \multicolumn{1}{c|}{433} \\ \cline{2-20} 
\end{tabular}%
}
\captionof{table}{True Positives (TP) and True Negatives (TN) for different benchmarks and part-of-speech}
\label{tab:wic-datasets}
\end{table*}

\begin{table*}
\centering
\resizebox{0.9\textwidth}{!}{%
\begin{tabular}{ccccccccccrrcc}
 &
  \textbf{} &
  \multicolumn{2}{c}{\textbf{WiC-en}} &
  \multicolumn{2}{c}{\textbf{MCL-WiC-en}} &
  \multicolumn{2}{c}{\textbf{XL-WiC-fr}} &
  \multicolumn{2}{c}{\textbf{XL-WiC-it}} &
  \multicolumn{2}{c}{\textbf{WiC-ITA-it}} &
  \multicolumn{2}{c}{\textbf{DWUG-de}} \\ \cline{3-14} 
 &
  \multicolumn{1}{c|}{Layer} &
  \textit{Train} &
  \multicolumn{1}{c|}{\textit{Test}} &
  \textit{Train} &
  \multicolumn{1}{c|}{\textit{Test}} &
  \textit{Train} &
  \multicolumn{1}{c|}{\textit{Test}} &
  \textit{Train} &
  \multicolumn{1}{c|}{\textit{Test}} &
  \multicolumn{1}{c}{\textit{Train}} &
  \multicolumn{1}{c|}{\textit{Test}} &
  \textit{Train} &
  \multicolumn{1}{c|}{\textit{Test}} \\ \cline{2-14} 
\multicolumn{1}{c|}{\multirow{3}{*}{\textbf{nouns}}} &
  \multicolumn{1}{c|}{\textit{1}} &
  \textbf{0.593} &
  \multicolumn{1}{c|}{\textbf{0.606}} &
  \textbf{0.656} &
  \multicolumn{1}{c|}{\textbf{0.727}} &
  \textbf{-} &
  \multicolumn{1}{c|}{\textbf{0.591}} &
  \textbf{0.642} &
  \multicolumn{1}{c|}{\textbf{0.679}} &
  \textbf{0.644} &
  \multicolumn{1}{r|}{\textbf{0.555}} &
  \textbf{0.808} &
  \multicolumn{1}{c|}{\textbf{0.799}} \\
\multicolumn{1}{c|}{} &
  \multicolumn{1}{c|}{\textit{6}} &
  \textbf{0.697} &
  \multicolumn{1}{c|}{\textbf{0.656}} &
  \textbf{0.720} &
  \multicolumn{1}{c|}{\textbf{0.812}} &
  \textbf{-} &
  \multicolumn{1}{c|}{\textbf{0.661}} &
  \multicolumn{1}{r}{\textbf{0.678}} &
  \multicolumn{1}{r|}{\textbf{0.713}} &
  0.694 &
  \multicolumn{1}{r|}{\textbf{0.699}} &
  \textbf{0.808} &
  \multicolumn{1}{c|}{\textbf{0.800}} \\
\multicolumn{1}{c|}{} &
  \multicolumn{1}{c|}{\textit{12}} &
  \textbf{0.691} &
  \multicolumn{1}{c|}{\textbf{0.683}} &
  \textbf{0.796} &
  \multicolumn{1}{c|}{\textbf{0.847}} &
  - &
  \multicolumn{1}{c|}{\textbf{0.677}} &
  \multicolumn{1}{r}{\textbf{0.678}} &
  \multicolumn{1}{r|}{\textbf{0.689}} &
  0.682 &
  \multicolumn{1}{r|}{\textbf{0.759}} &
  \textbf{0.806} &
  \multicolumn{1}{c|}{\textbf{0.809}} \\ \cline{2-14} 
\multicolumn{1}{c|}{\multirow{3}{*}{\textbf{verbs}}} &
  \multicolumn{1}{c|}{\textit{1}} &
  0.558 &
  \multicolumn{1}{c|}{0.513} &
  0.572 &
  \multicolumn{1}{c|}{0.606} &
  \textbf{-} &
  \multicolumn{1}{c|}{0.530} &
  0.569 &
  \multicolumn{1}{c|}{0.562} &
  0.478 &
  \multicolumn{1}{r|}{0.539} &
  0.597 &
  \multicolumn{1}{c|}{0.597} \\
\multicolumn{1}{c|}{} &
  \multicolumn{1}{c|}{\textit{6}} &
  0.657 &
  \multicolumn{1}{c|}{0.613} &
  0.683 &
  \multicolumn{1}{c|}{0.782} &
  \textbf{-} &
  \multicolumn{1}{c|}{0.561} &
  \multicolumn{1}{r}{0.581} &
  \multicolumn{1}{r|}{0.582} &
  0.575 &
  \multicolumn{1}{r|}{0.586} &
  0.643 &
  \multicolumn{1}{c|}{0.633} \\
\multicolumn{1}{c|}{} &
  \multicolumn{1}{c|}{\textit{12}} &
  0.615 &
  \multicolumn{1}{c|}{0.611} &
  0.752 &
  \multicolumn{1}{c|}{0.805} &
  - &
  \multicolumn{1}{c|}{0.622} &
  \multicolumn{1}{r}{0.639} &
  \multicolumn{1}{r|}{0.593} &
  0.459 &
  \multicolumn{1}{r|}{0.615} &
  0.630 &
  \multicolumn{1}{c|}{0.640} \\ \cline{2-14} 
\multicolumn{1}{c|}{\textbf{adjectives}} &
  \multicolumn{1}{c|}{\textit{1}} &
  \textbf{-} &
  \multicolumn{1}{c|}{\textbf{-}} &
  0.650 &
  \multicolumn{1}{c|}{0.699} &
  \textbf{-} &
  \multicolumn{1}{c|}{0.539} &
  \textbf{-} &
  \multicolumn{1}{c|}{\textbf{-}} &
  0.666 &
  \multicolumn{1}{r|}{0.653} &
  \textbf{-} &
  \multicolumn{1}{c|}{\textbf{-}} \\
\multicolumn{1}{c|}{\textbf{}} &
  \multicolumn{1}{c|}{\textit{6}} &
  \textbf{-} &
  \multicolumn{1}{c|}{\textbf{-}} &
  0.703 &
  \multicolumn{1}{c|}{0.789} &
  \textbf{-} &
  \multicolumn{1}{c|}{0.574} &
  \textbf{-} &
  \multicolumn{1}{c|}{\textbf{-}} &
  \textbf{0.706} &
  \multicolumn{1}{r|}{0.687} &
  \textbf{-} &
  \multicolumn{1}{c|}{\textbf{-}} \\
\multicolumn{1}{c|}{} &
  \multicolumn{1}{c|}{\textit{12}} &
  - &
  \multicolumn{1}{c|}{-} &
  0.738 &
  \multicolumn{1}{c|}{0.819} &
  - &
  \multicolumn{1}{c|}{0.653} &
  - &
  \multicolumn{1}{c|}{-} &
  \textbf{0.733} &
  \multicolumn{1}{r|}{0.695} &
  - &
  \multicolumn{1}{c|}{-} \\ \cline{2-14} 
\end{tabular}%
}
\caption{\textbf{BERT}: Comparison of F1 score scores obtained by threshold-based classifiers for Word in Context (WiC) trained on development sets. The threshold is determined on the development set and applied to both the train and test sets. Results are provided for different parts of speech and WiC benchmarks. We report in bold the best result for each considered layer, benchmark, and data sets.}
\label{tab:bert-wic-roc}
\end{table*}

\begin{table*}
\centering
\resizebox{0.9\textwidth}{!}{%
\begin{tabular}{ccccccccccrrcc}
 &
  \textbf{} &
  \multicolumn{2}{c}{\textbf{WiC-en}} &
  \multicolumn{2}{c}{\textbf{MCL-WiC-en}} &
  \multicolumn{2}{c}{\textbf{XL-WiC-fr}} &
  \multicolumn{2}{c}{\textbf{XL-WiC-it}} &
  \multicolumn{2}{c}{\textbf{WiC-ITA-it}} &
  \multicolumn{2}{c}{\textbf{DWUG-de}} \\ \cline{3-14} 
 &
  \multicolumn{1}{c|}{Layer} &
  \textit{Train} &
  \multicolumn{1}{c|}{\textit{Test}} &
  \textit{Train} &
  \multicolumn{1}{c|}{\textit{Test}} &
  \textit{Train} &
  \multicolumn{1}{c|}{\textit{Test}} &
  \textit{Train} &
  \multicolumn{1}{c|}{\textit{Test}} &
  \multicolumn{1}{c}{\textit{Train}} &
  \multicolumn{1}{c|}{\textit{Test}} &
  \textit{Train} &
  \multicolumn{1}{c|}{\textit{Test}} \\ \cline{2-14} 
\multicolumn{1}{c|}{\multirow{3}{*}{\textbf{nouns}}} &
  \multicolumn{1}{c|}{\textit{1}} &
  0.530 &
  \multicolumn{1}{c|}{0.521} &
  \textbf{0.592} &
  \multicolumn{1}{c|}{\textbf{0.632}} &
  \textbf{-} &
  \multicolumn{1}{c|}{\textbf{0.588}} &
  \textbf{0.612} &
  \multicolumn{1}{c|}{\textbf{0.645}} &
  0.571 &
  \multicolumn{1}{r|}{0.582} &
  \textbf{0.819} &
  \multicolumn{1}{c|}{\textbf{0.811}} \\
\multicolumn{1}{c|}{} &
  \multicolumn{1}{c|}{\textit{6}} & %%%%6
  \textbf{0.624} &
  \multicolumn{1}{c|}{\textbf{0.628}} &
  0.675 &
  \multicolumn{1}{c|}{\textbf{0.738}} &
  \textbf{-} &
  \multicolumn{1}{c|}{\textbf{0.625}} &
  \multicolumn{1}{r}{\textbf{0.690}} &
  \multicolumn{1}{r|}{\textbf{0.675}} &
  0.691 &
  \multicolumn{1}{r|}{0.691} &
  \textbf{0.807} &
  \multicolumn{1}{c|}{\textbf{0.794}} \\
\multicolumn{1}{c|}{} &
  \multicolumn{1}{c|}{\textit{12}} &
  \textbf{0.644} &
  \multicolumn{1}{c|}{\textbf{0.611}} &
  0.705 &
  \multicolumn{1}{c|}{\textbf{0.780}} &
  - &
  \multicolumn{1}{c|}{\textbf{0.707}} &
  \multicolumn{1}{r}{\textbf{0.644}} &
  \multicolumn{1}{r|}{\textbf{0.680}} &
  \textbf{0.691} &
  \multicolumn{1}{r|}{\textbf{0.713}} &
  \textbf{0.813} &
  \multicolumn{1}{c|}{\textbf{0.812}} \\ \cline{2-14} 
\multicolumn{1}{c|}{\multirow{3}{*}{\textbf{verbs}}} &
  \multicolumn{1}{c|}{\textit{1}} &
  \textbf{0.563} &
  \multicolumn{1}{c|}{\textbf{0.547}} &
  0.564 &
  \multicolumn{1}{c|}{0.576} &
  \textbf{-} &
  \multicolumn{1}{c|}{0.520} &
  0.562 &
  \multicolumn{1}{c|}{0.524} &
  0.477 &
  \multicolumn{1}{r|}{0.601} &
  0.618 &
  \multicolumn{1}{c|}{0.617} \\
\multicolumn{1}{c|}{} &
  \multicolumn{1}{c|}{\textit{6}} &
  0.604 &
  \multicolumn{1}{c|}{0.555} &
   0.622   &
  \multicolumn{1}{c|}{0.682} &
  \textbf{-} &
  \multicolumn{1}{c|}{0.571} &
  \multicolumn{1}{r}{0.596} &
  \multicolumn{1}{r|}{0.554} &
  0.555 &
  \multicolumn{1}{r|}{0.566} &
  0.669 &
  \multicolumn{1}{c|}{0.627} \\
\multicolumn{1}{c|}{} &
  \multicolumn{1}{c|}{\textit{12}} &
  0.623 &
  \multicolumn{1}{c|}{0.586} &
  0.698 &
  \multicolumn{1}{c|}{0.720} &
  - &
  \multicolumn{1}{c|}{0.662} &
  \multicolumn{1}{r}{0.552} &
  \multicolumn{1}{r|}{0.543} &
  0.578 &
  \multicolumn{1}{r|}{0.506} &
  0.667 &
  \multicolumn{1}{c|}{0.675} \\ \cline{2-14} 
\multicolumn{1}{c|}{\textbf{adjectives}} &
  \multicolumn{1}{c|}{\textit{1}} &
  \textbf{-} &
  \multicolumn{1}{c|}{\textbf{-}} &
  0.548 &
  \multicolumn{1}{c|}{0.568} &
  \textbf{-} &
  \multicolumn{1}{c|}{0.531} &
  \textbf{-} &
  \multicolumn{1}{c|}{\textbf{-}} &
  \textbf{0.633} &
  \multicolumn{1}{r|}{\textbf{0.614}} &
  \textbf{-} &
  \multicolumn{1}{c|}{\textbf{-}} \\
\multicolumn{1}{c|}{\textbf{}} &
  \multicolumn{1}{c|}{\textit{6}} &
  \textbf{-} &
  \multicolumn{1}{c|}{\textbf{-}} &
   \textbf{0.676} &
  \multicolumn{1}{c|}{0.736} &
  \textbf{-} &
  \multicolumn{1}{c|}{0.598} &
  \textbf{-} &
  \multicolumn{1}{c|}{\textbf{-}} &
  \textbf{0.715} &
  \multicolumn{1}{r|}{\textbf{0.750}} &
  \textbf{-} &
  \multicolumn{1}{c|}{\textbf{-}} \\
\multicolumn{1}{c|}{} &
  \multicolumn{1}{c|}{\textit{12}} &
  - &
  \multicolumn{1}{c|}{-} &
  \textbf{0.707} &
  \multicolumn{1}{c|}{0.735} &
  - &
  \multicolumn{1}{c|}{0.701} &
  - &
  \multicolumn{1}{c|}{-} &
  0.600 &
  \multicolumn{1}{r|}{0.683} &
  - &
  \multicolumn{1}{c|}{-} \\ \cline{2-14} 
\end{tabular}%
}
\caption{\textbf{mBERT}: Comparison of F1 score scores obtained by threshold-based classifiers for Word in Context (WiC) trained on development sets. The threshold is determined on the development set and applied to both the train and test sets. Results are provided for different parts of speech and WiC benchmarks. We report in bold the best result for each considered layer, benchmark, and data sets.}
\label{tab:mbert-wic-roc}
\end{table*}

\section{Word-in-Context (WiC)}\label{app:wic}
In the WiC experiments, we leveraged pre-trained models without performing any kind of fine-tuning (therefore not using the Train set). The Dev set, as in traditional experimental settings, was used to tune the only parameter involved in our experiments: the threshold used to determine if the words in the two sentences have the same meaning or not. In other words, pairs of examples for which the cosine similarity is lower than the threshold are classified as negative; otherwise, they are classified as positive. In our experiments, we follow~\newcite{pilehvar2019wic} in tuning the threshold-based classifier on the development set (Dev), thus being able to compare with their results. Additionally, for French, a Train set is not available. PoS-specific thresholds have been computed to guarantee a fair evaluation across different PoS tags. Regarding the size of the PoS-specific sets, we argue that the number of examples, even if small, is sufficient to establish a binary threshold. This is supported by our results across different datasets, which achieve comparable outcomes to the SOTA result on the full set (not PoS split, as shown in Table~\ref{tab:wic-roc}). We would like to highlight that similar results are obtained when using the Train set instead of the Dev set for the threshold selection.

\subsection{The DWUG benchmark}
In the original SemEval DWUG benchmarks~\cite{schlechtweg2020semeval}, human annotators were provided with a target word and a pair of sentences and asked to estimate the degree of change on a scale from 1 (change) to 4 (identical). The task is analogue to a multi-class WiC task. We converted the original annotations to a binary WiC benchmark. Specifically, we transformed the ground truth for a specific pair of sentences as follows: if the average agreement of the Lexical Semantic Change annotations was greater than 3.5, we considered the meaning to be the same (assigned a label of 1); for sentence pairs with an average agreement lower than 1.5, we considered the meaning to be different (assigned a label of 0).

\subsection{Size of WiC benchmarks}\label{app:DWUG}
We split the considered WiC benchmarks in distinct sub-corpora for nouns, verbs, and adjectives. In Table\ref{tab:wic-datasets}, we provide the number of true (i.e. 1, same meaning) and negative (i.e. 0, different meaning) instances for each sub-corpus.

\subsection{Macro-F1 across BERT layers}
We examine the PoS sensitivity using WiC by comparing embedding similarities across all BERT and mBERT layers. For sake of simplicity, we provide additional results using Macro F1-score for layers 1, 6, and 12 across various PoS categories and corpora. Results are consistent across the layers, confirming the best performance for the noun syntactic class. We have omitted the WiC results for XLM-R due to its tokenisation characteristics. For numerous pairs of sentences, the XLM-R tokeniser generates more tokens than BERT and mBERT, surpassing the input limit and causing the exclusion of target words. 

\newpage

\section{WiC polysemy per language}\label{app:polysemy}
\begin{minipage}{\textwidth}
\centering
   \includegraphics[width=\textwidth]{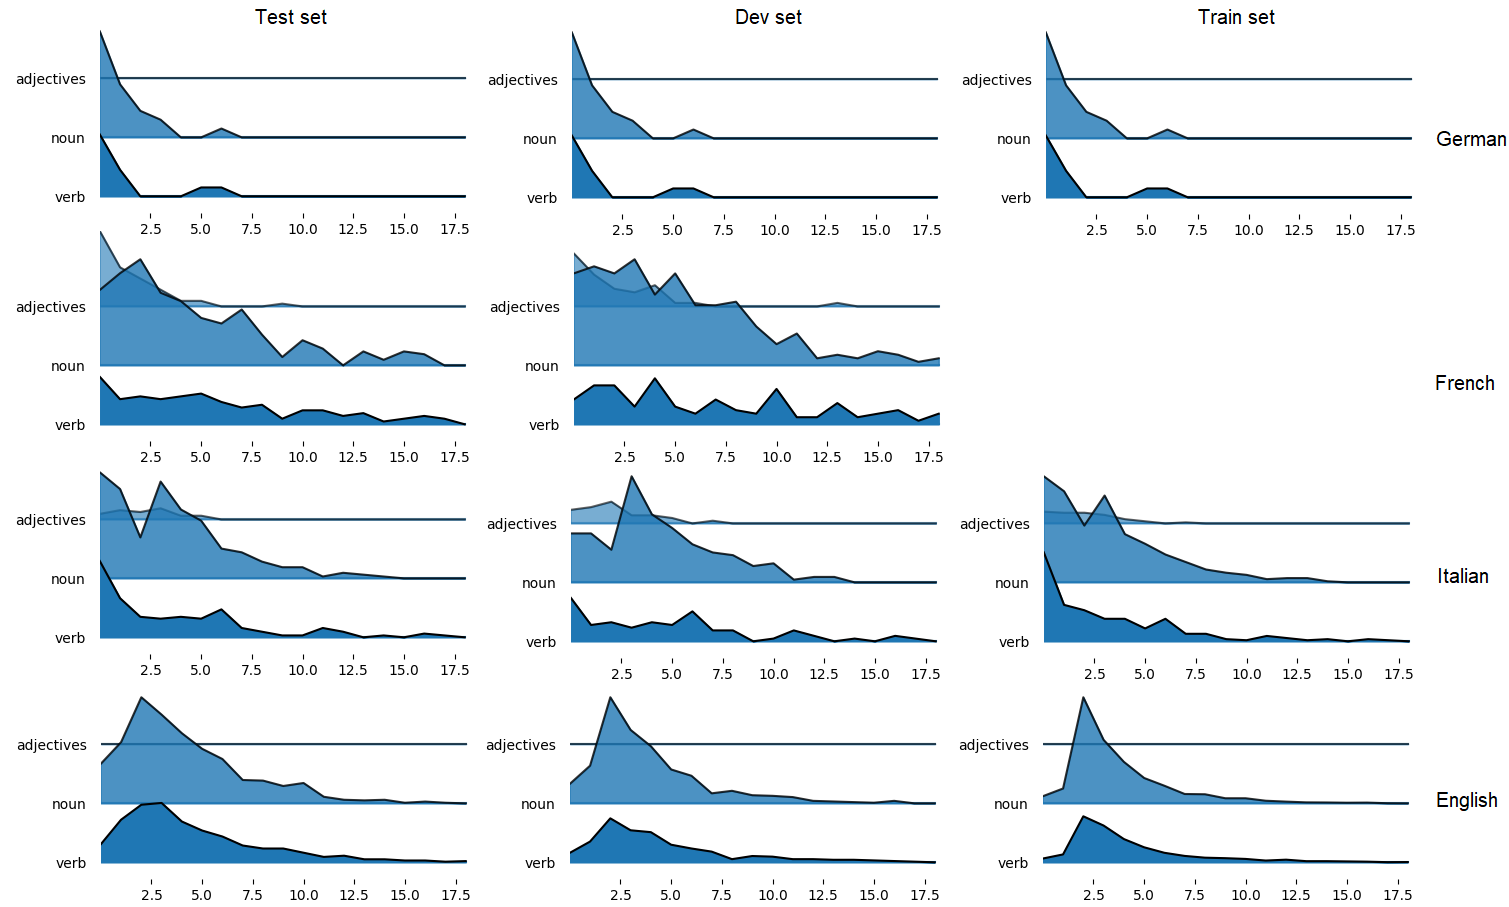}
   \captionof{figure}{Distribution of polysemy (i.e., number of senses on x-axis) of the target words in each Dev, Test, and Train WiC set for each considered language}
   \label{fig:full-polysemy}
\end{minipage}

\begin{comment}
\section{Models}
\label{app:hyper}
\begin{minipage}[t]{\columnwidth}
\centering
\begin{tabular}{ |l|l| }
\hline
\textbf{Model}
& \textbf{HF Identifier}\\
\hline
monolingual BERT & bert-base-uncased\\
\hline
mBER & bert-base-multilingual-cased\\
\hline
XLM-R & xlm-roberta-base\\
\hline
\end{tabular}
\captionof{table}{Model identifier in the HuggingFace Hub.}
\label{tag:hyper-params}
\end{minipage}
\end{comment}

\begin{table}[!ht]
\centering
\resizebox{\columnwidth}{!}{%
\begin{tabular}{ccc}
\textbf{References} & \textbf{Benchmark} & \textbf{\# targets} \\
\citealp{schlechtweg2020semeval} & DWUG-English & 46 \\
\citealp{schlechtweg2020semeval} & DWUG-German & 50 \\
\citealp{schlechtweg2020semeval} & DWUG-Swedish & 44 \\
\citealp{zamora2022lscdiscovery} & DWUG-Spanish & 100
\end{tabular}%
}
\caption{References and number of targets for each consider artificial corpus}
\label{tab:artificial-corpora}
\end{table}

\clearpage

\section{\texttt{Random} Lexical Semantic Change}\label{app:synthetic-LSC}
\subsection{Artificial diachronic corpus}
We generated an artificial diachronic corpus for LSC by utilising the SemEval and LSCDiscovery benchmakrs for LSC in DWUG format\footnote{English: \url{https://zenodo.org/records/5796878}, German: \url{https://zenodo.org/records/5796871}, Swedish: \url{https://zenodo.org/records/5090648}, Spanish: \url{https://zenodo.org/records/6433667}} (see Table \ref{tab:artificial-corpora}). Instead of incorporating data from both time periods, $T_1$ and $T_2$, we discarded information from the first time period as it is more likely to contain word meanings outside the pre-trained knowledge of the models under examination. We created two distinct artificial sub-corpora, $C_1$ and $C_2$, by randomly sampling occurrences from the data of the second time period $T_2$. The DWUG English dataset contains data for 46 target words.

For each target $t$, we considered all sentences where another target $t1$, with $t1 \neq t$, appeared as potential candidates to emulate instances of semantic change. We simulated a change instance through a \textit{random} replacement, that is by replacing $t$ in the sentence where $t1$ occurred -- i.e., $t1 \leftarrow t$. We sample a varying number of sentences and perform replacements for each target, thereby emulating a varying degree of semantic change. 

\begin{figure}[!h]
 \centering
    \includegraphics[width=\columnwidth]{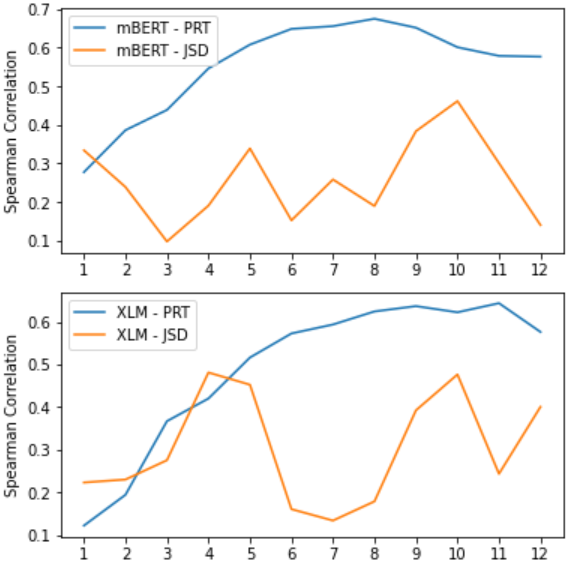}
    \captionof{figure}{PRT and JSD performance on the artificial LSC dataset}
    \label{fig:random-LSC-models}
 \end{figure}

\section{Lexical Semantic Change}

\begin{minipage}[t]{\columnwidth}
\centering
\resizebox{\columnwidth}{!}{%
\begin{tabularx}{5.5in}{|l|l|X|r|}
\hline
Word                    & Time span & (Ranked) Farthest replacements                                                                                                    & \multicolumn{1}{l|}{$lsc_w$ (k=1)} \\ \hline
\multirow{2}{*}{attack} & T1        & \textbf{physical}, degeneration, blast, crime, disease, death, condition, plane, affliction, birthday attack                                     & -0.036                      \\ \cline{2-4} 
                        & T2        & \textbf{approach}, force, onslaught, assault, exploit, challenge, commencement, aim, worth, signal                                               & 0.059                       \\ \hline
\multirow{2}{*}{bit}    & T1        & \textbf{nominative case}, accusative case, cryptography, information theory, bdsm, time,point, binary digit, sociologic, sublative              & -0.018                   \\ \cline{2-4} 
                        & T2        & \textbf{saddlery}, chard, illative case, iron, bevelled, tack, small, gun, cut, elative case                                                     & 0.067                       \\ \hline
\multirow{2}{*}{circle} & T1        & \textbf{wicca}, circumlocution, encircle, astronomy, tavern, semicircle, around, logic, go,wand                                                 & 0.002                    \\ \cline{2-4} 
                        & T2        & \textbf{pitch}, place, graduated, figure, disk, territorial, enforce, worship, line, bagginess                                                   & 0.064                      \\ \hline
\multirow{2}{*}{edge}   & T1        & \textbf{brink}, cricket, instrument, margin, polytope, side, edge computing, verge, demarcation line, demarcation                                & -0.015                      \\ \cline{2-4} 
                        & T2        & \textbf{data}, production, climax, division, superiority, organization, sharpness, graph, win, geometry                                          & 0.047                      \\ \hline
\multirow{2}{*}{graft}  & T1        & \textbf{lesion}, bribery, felony, politics, bribe, corruption, autoplasty, surgery, nautical, illicit                                            & -0.047                     \\ \cline{2-4} 
                        & T2        & \textbf{branch}, stock, tree, fruit, shoot, join, cut, graft the forked tree, stem, portion                                                      & 0.103                      \\ \hline
\multirow{2}{*}{head}   & T1        & \textbf{headland}, head word, capitulum, syntactic, pedagogue, fluid dynamics, hip hop, headway, pedagog, word                                   & 0.004                      \\ \cline{2-4} 
                        & T2        & \textbf{leader}, organs, implement, top, tail, foreland, chief, bolt, axe, forefront                                                             & 0.084                     \\ \hline
\multirow{2}{*}{land}   & T1        & \textbf{real estate}, real property, surface, property,build, physical object, Edwin Herbert Land, electronics, landing, first person           & -0.032                      \\ \cline{2-4} 
                        & T2        & \textbf{realm}, country, kingdom, province, domain, people, homeland, territory, nation, region                                                  & 0.076                      \\ \hline
\multirow{2}{*}{lass}   & T1        & \textbf{sweetheart}, girl, missy, woman, yorkshire, lassem, lasst, lassie, loss, miss                                                            & 0.014                      \\ \cline{2-4} 
                        & T2        & \textbf{fille}, dative case, jeune fille, loose, lasses, unattached, young lady, young woman, north east england, past participle                & 0.099                    \\ \hline
\multirow{2}{*}{plane}  & T1        & \textbf{airplane}, aeroplane, pt boat, heavier-than-air craft, glide , boat, lycaenidae, lift, bow, hand tool                                     & -0.197                   \\ \cline{2-4} 
                        & T2        & \textbf{geometry}, point, shape, surface, flat, degree, form, range, anatomy, smooth                                                             & 0.205                  \\ \hline
\multirow{2}{*}{player} & T1        & \textbf{media player}, idler, soul, thespian, person, individual, trifler, performer, somebody, histrion                                         & -0.065                      \\ \cline{2-4} 
                        & T2        & \textbf{contestant}, performing artist, actor, musician, musical instrument, music, gamer, theater, player piano, play the field                 & 0.042                      \\ \hline
\multirow{2}{*}{prop}   & T1        & \textbf{props}, airscrew, astronautics, actor, airplane propeller, seashell, stagecraft, stage, property, art                                    & -0.042                    \\ \cline{2-4} 
                        & T2        & \textbf{around}, rugby, imperative mood, about, singular, scrum, ignition, roughly, ballot, manually                                             & 0.088                      \\ \hline
\multirow{2}{*}{rag}    & T1        & \textbf{ragtime}, nominative case, accusative case, rag week, terminative case, inflectional, sublative, piece of material, tag, sanitary napkin & -0.049                      \\ \cline{2-4} 
                        & T2        & \textbf{clothes}, exhaustion, university, society, silk, ragged, journalism, haze, ranking, torment                                              & 0.071                     \\ \hline
\multirow{2}{*}{record} & T1        & \textbf{attainment}, track record, achievement, accomplishment, struct, number, intransitive, record book, criminal record, disc                 & -0.036                     \\ \cline{2-4} 
                        & T2        & \textbf{evidence}, document, information, audio, recollection, storage medium, memory, electronic, sound recording, data                         & 0.089                     \\ \hline
\multirow{2}{*}{stab}   & T1        & \textbf{thread}, staccato, feeling, nominative case, sheet, chord, bacterial, culture, twinge, sensation                                         & -0.046                     \\ \cline{2-4} 
                        & T2        & \textbf{wound}, tool, knife thrust, weapon, plaster, criticism, wire, pierce, thrust, try                                                        & 0.029                     \\ \hline
\multirow{2}{*}{thump}  & T1        & \textbf{clunk}, throb, clump, thud, pound, thumping, rhythmic, sound, blow, hit                                                                  & -0.036                    \\ \cline{2-4} 
                        & T2        & \textbf{muffled}, hit, blow, sound, rhythmic, thumping, pound, thud, clump, throb                                                                & 0.033                     \\ \hline
\multirow{2}{*}{tip}    & T1        & \textbf{gratuity}, first person, forty, bloke, singular, overturn, stringed instrument, unbalanced, taxi driver, sated                           & -0.031                      \\ \cline{2-4} 
                        & T2        & \textbf{brush}, tap, strike, gift, tram, flex, tumble, heap, full, hint                                                                          & 0.070                     \\ \hline
\end{tabularx}%
}
\captionof{table}{Words annotated as changed in SemEval 2020 Task 1: Binary Subtask and retrieved farthest replacements for each time span.}
\label{ref:eng_changes}
\end{minipage}

\clearpage

\begin{figure*}[!h]
 \centering
    \includegraphics[width=\textwidth]{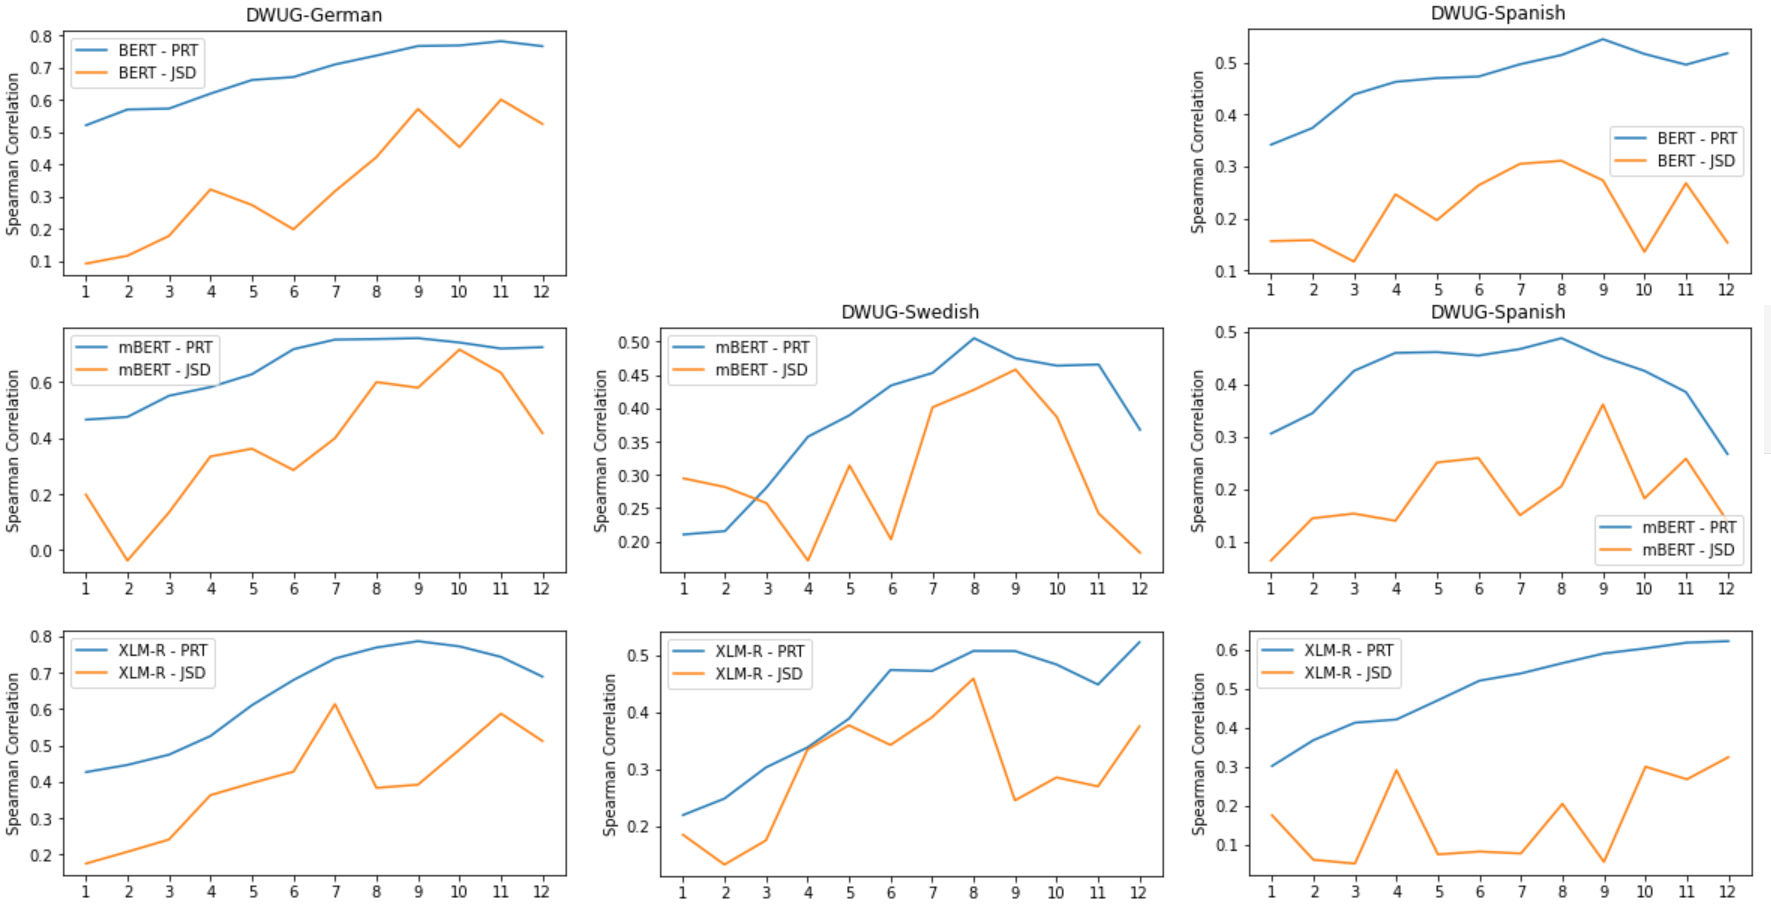}
    \captionof{figure}{PRT and JSD performance on the artificial LSC dataset}
    \label{fig:random-LSC-languages}
 \end{figure*}
